# Supplementary material for: Thermodynamics of surfactant-enriched binary-fluid systems
Source: arXiv:2405.17482 source file (2024-05-24)
Supplement: Supplementary file 1 [file Graphical_abstract.tex]

\section{Graphical Abstract}
\begin{figure}[h]
    \centering
    \includegraphics[width=\textwidth]{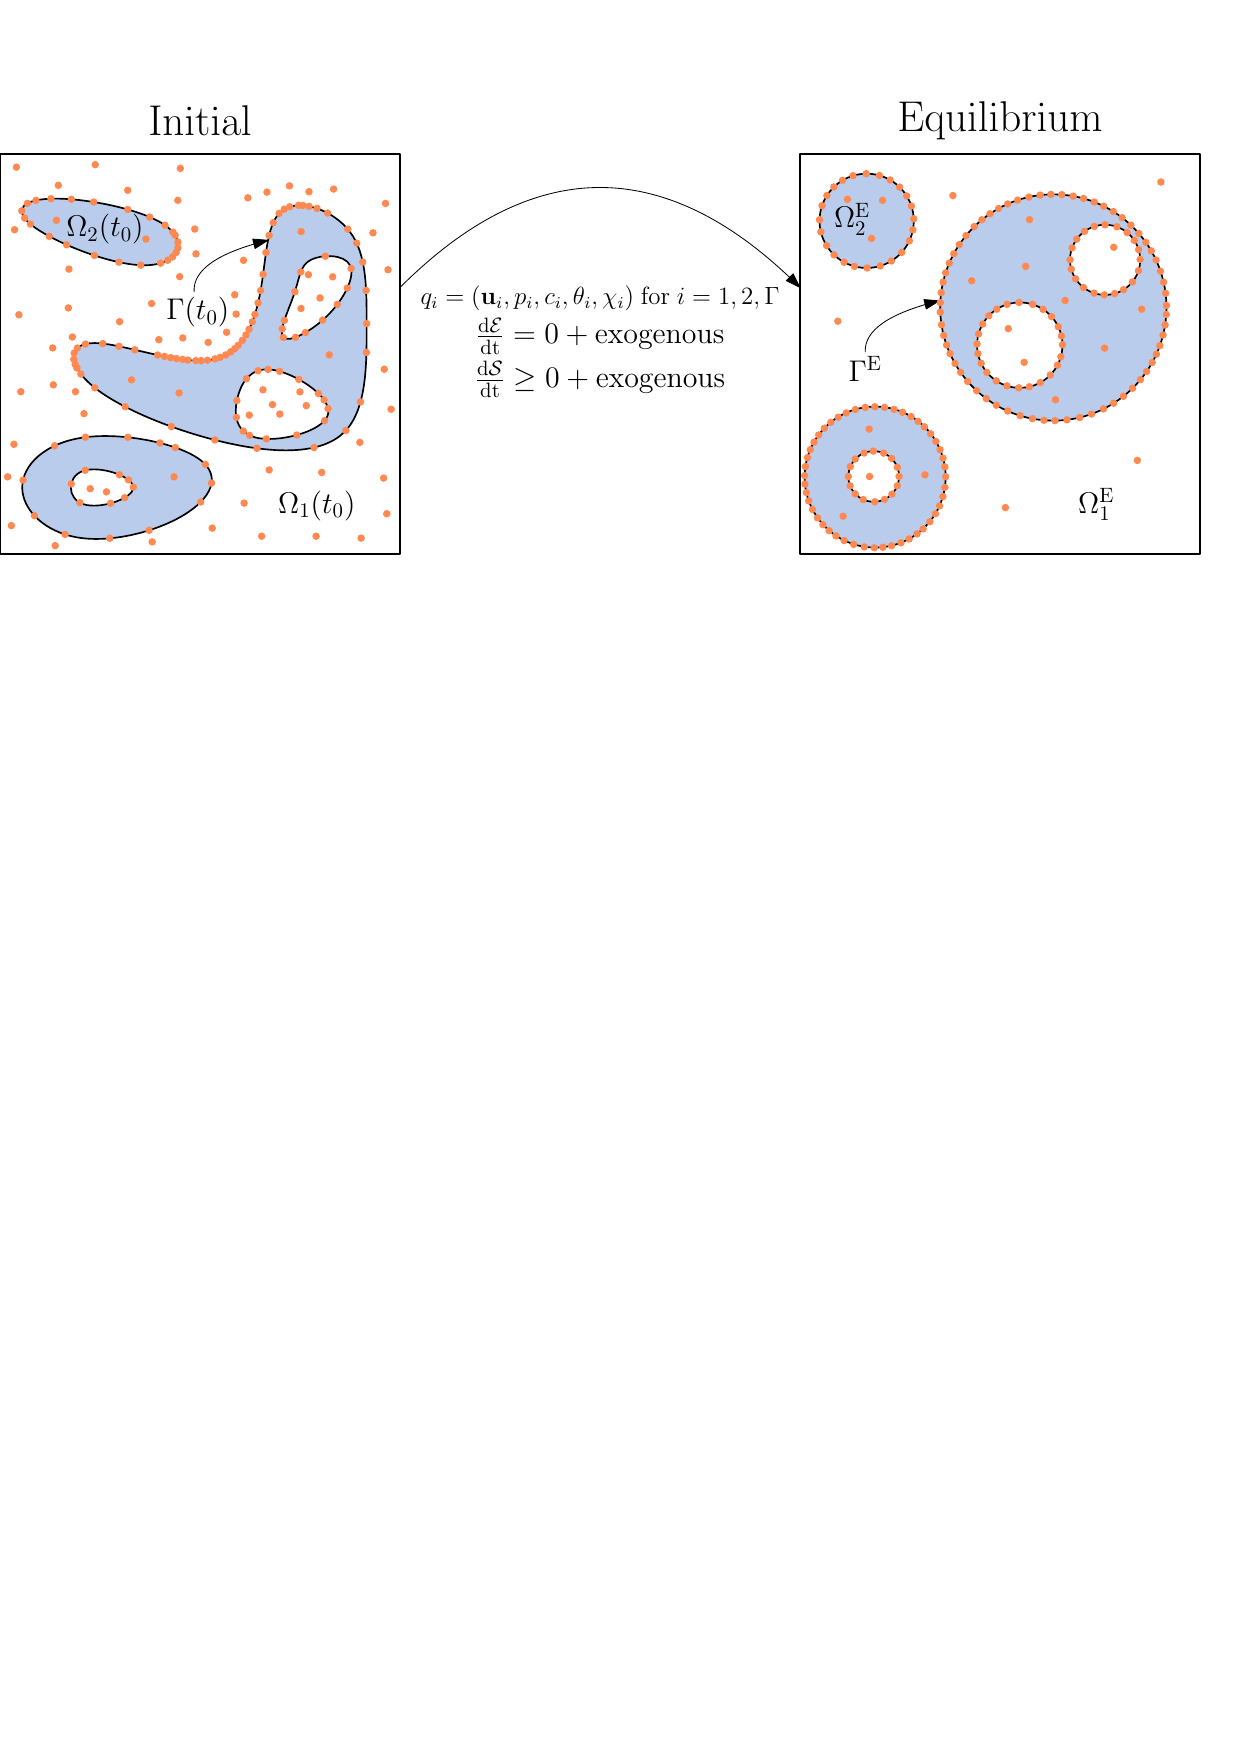}
    \caption{For Table of Contents Only}
    \label{fig:graphicalabstract}
\end{figure}
